# Supplementary material for: Predicting the Big Five Personality Traits in Chinese Counselling Dialogues Using Large Language Models
Source: arXiv:2406.17287 source file (2024-06-25)
Supplement: Supplementary file 1 [file appendix.tex]

% \appendix

% \section{Appendices}

% \subsection{Ablation Study}

% % \subsubsection{Effect of different LLMs}

% \begin{figure*}[ht]
%     \centering
%     \includegraphics[width=\textwidth]{figures/correlation_LLMs.png}
%     \caption{Correlation between predicted and actual Big Five traits using different LLMs.}
%     \label{fig:correlation_LLMs}
% \end{figure*}

% % \subsubsection{Effect of model size}

% \begin{figure*}[ht]
%     \centering
%     \includegraphics[width=\textwidth]{figures/correlation_model_size.png}
%     \caption{Effect of model size of Qwen1.5 serires on the performance of predicting Big Five traits.}
%     \label{fig:correlation-modelsize}
% \end{figure*}
